# Supplementary material for: Learning Transformations To Reduce the Geometric Shift in Object Detection
Source: arXiv:2301.05496 source file (2023-01-13)
Supplement: Supplementary file 2 [file supp_da.tex]

\begin{table}[h]

  \centering
  \begin{tabular}{lcc}
    \toprule

    Method     & Car AP@0.5 & Pedestrian AP@0.5 \\
    \midrule
    ~\cite{li2022cross} & 77.2 & 63.5\\
    Ours(N=9) & 80.4\tiny{$\pm$0.15} & Ours(N=5) 65.3\tiny{$\pm$ 0.37}\\
    \bottomrule
  \end{tabular}
    \caption{FoV Adaptation }
      \label{tab:supp_da}
\end{table}
