# Supplementary material for: Learning Transformations To Reduce the Geometric Shift in Object Detection
Source: arXiv:2301.05496 source file (2023-01-13)
Supplement: Supplementary file 3 [file supp_tau_lamda.tex]

% !TEX root = ../supp.tex
% !TEX spellcheck = en-US
\begin{table}[h]
  \caption{Mean Teacher Training }
  \label{tab:supp_tau_lamda}
  \centering
  \begin{tabular}{lc}
    \toprule

    Kind     & Details  \\
    \midrule
    Random Crop & Relative Range: $[0.3 ,1]$ \\

    Color Jitter & Brightness=$.5$, Hue=$.3$\\
    \bottomrule
  \end{tabular}
\end{table}
